# Supplementary material for: Cross-View Image Sequence Geo-localization
Source: arXiv:2210.14295 source file (2022-11-02)

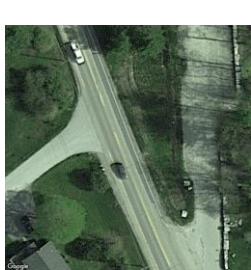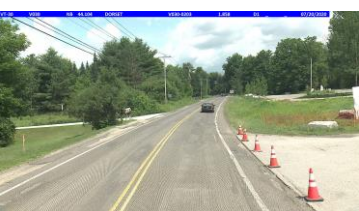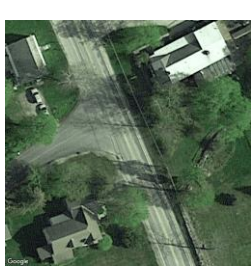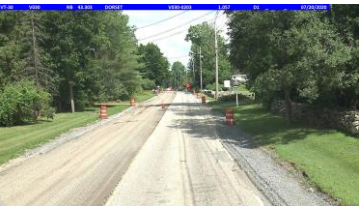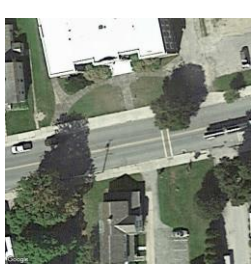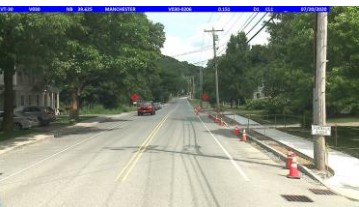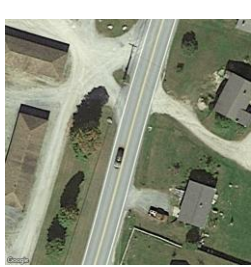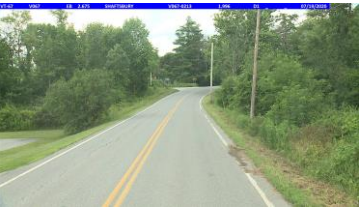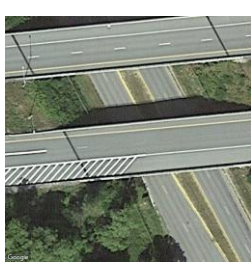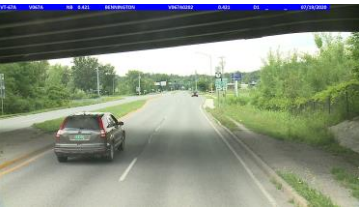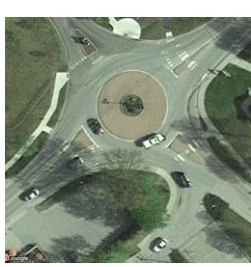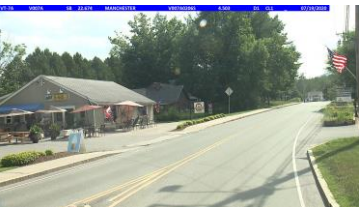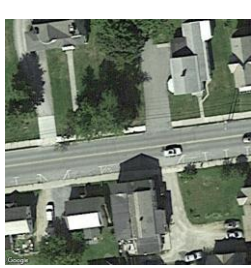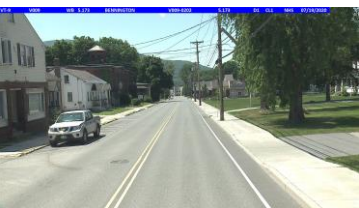



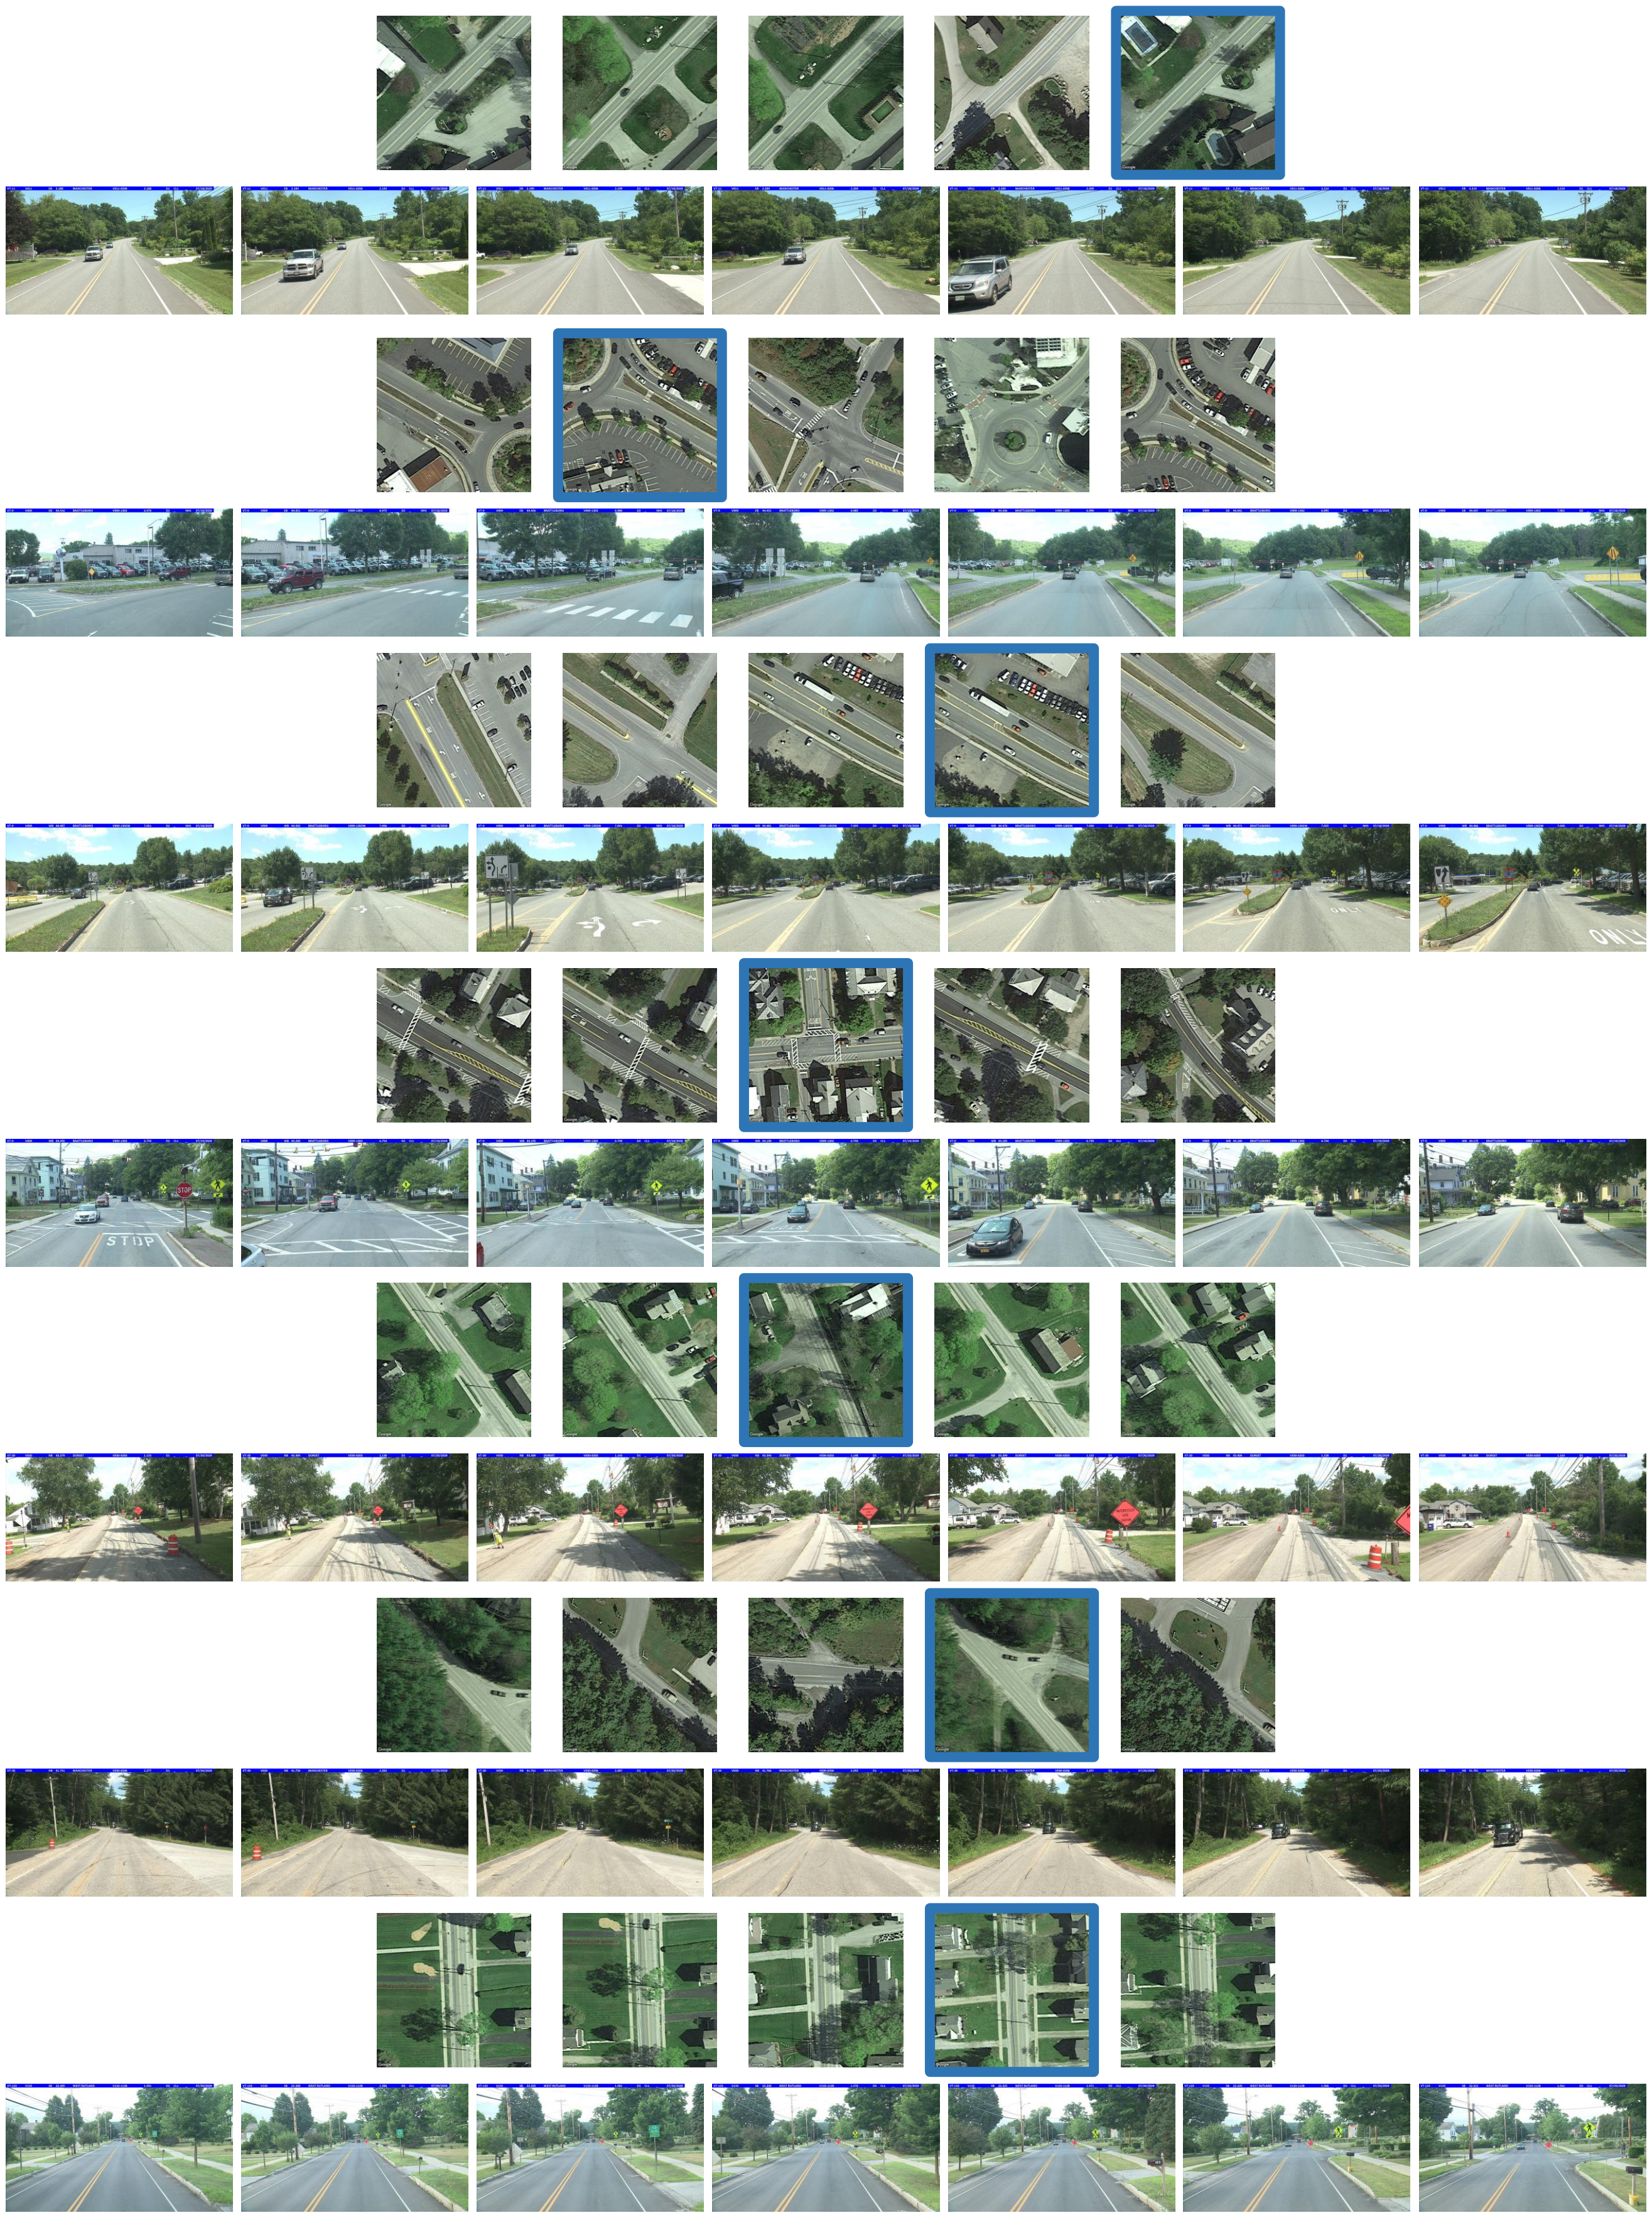



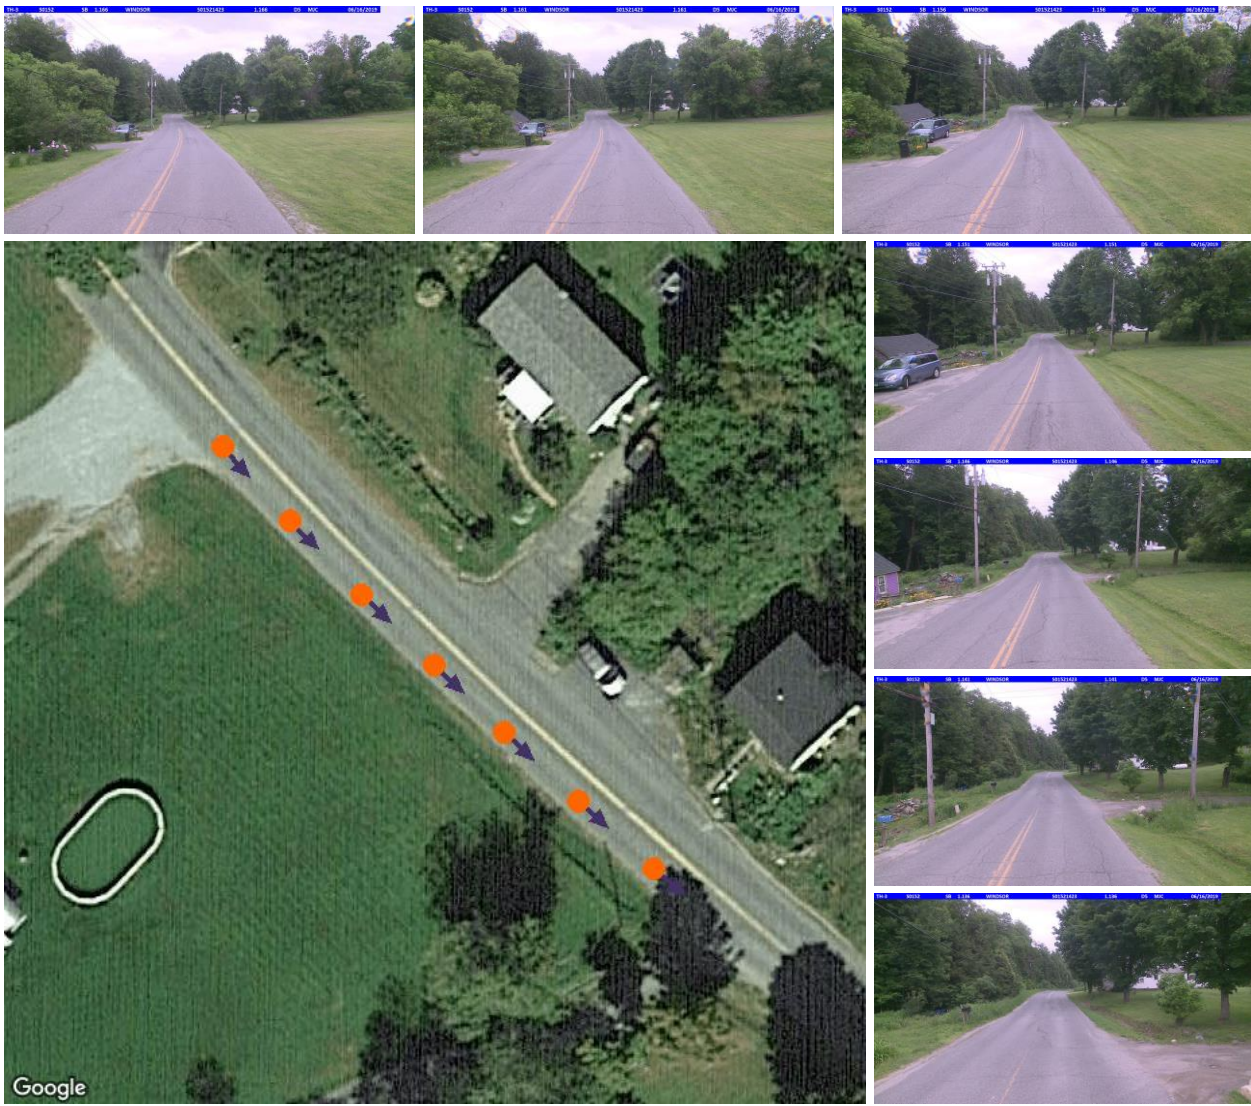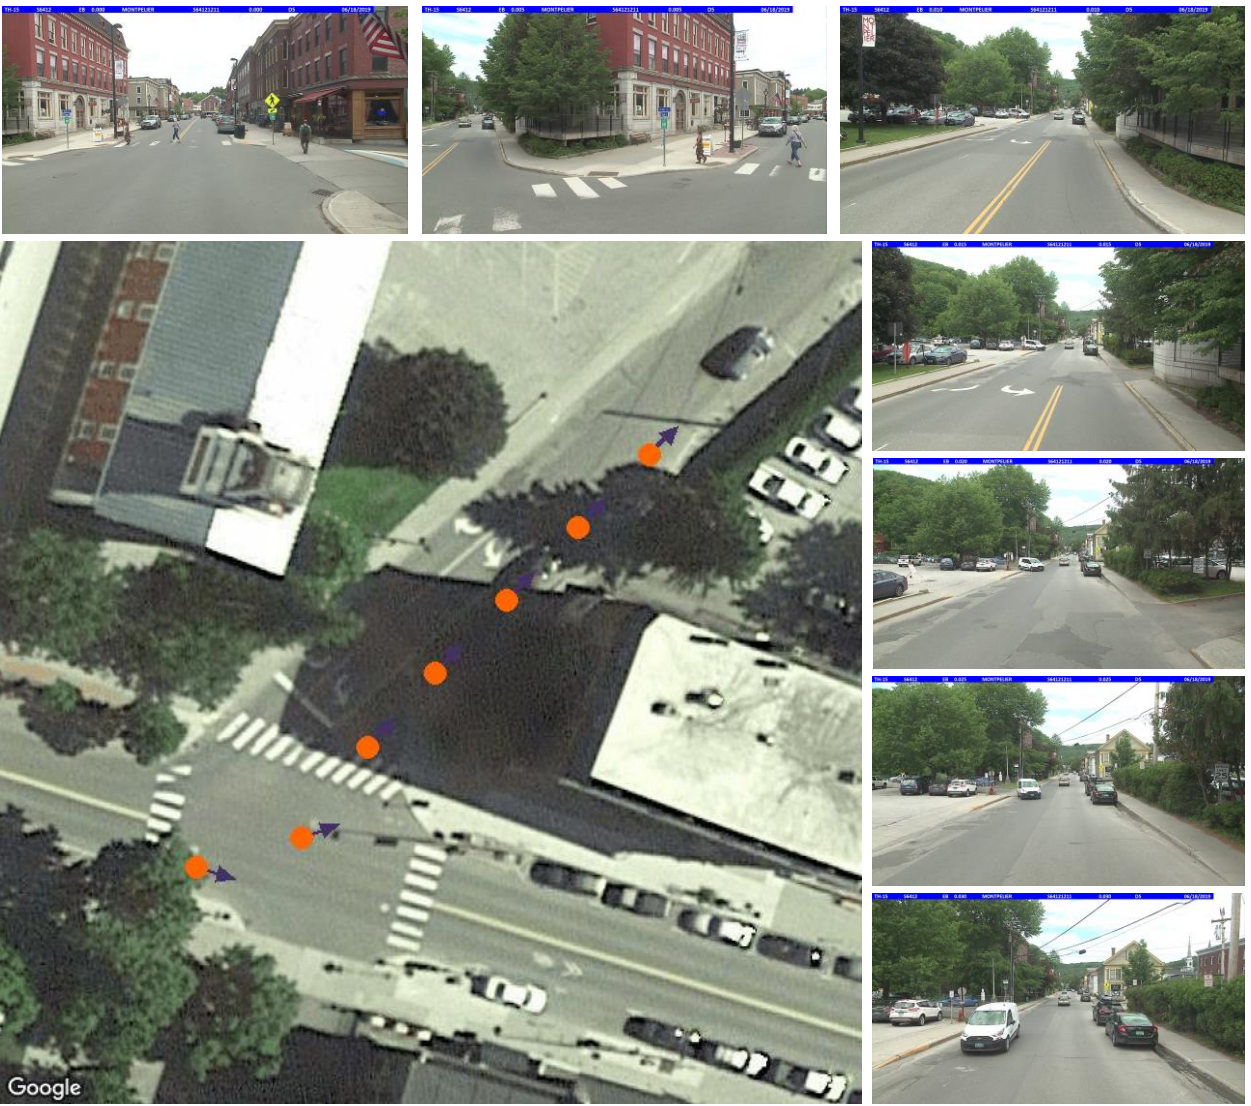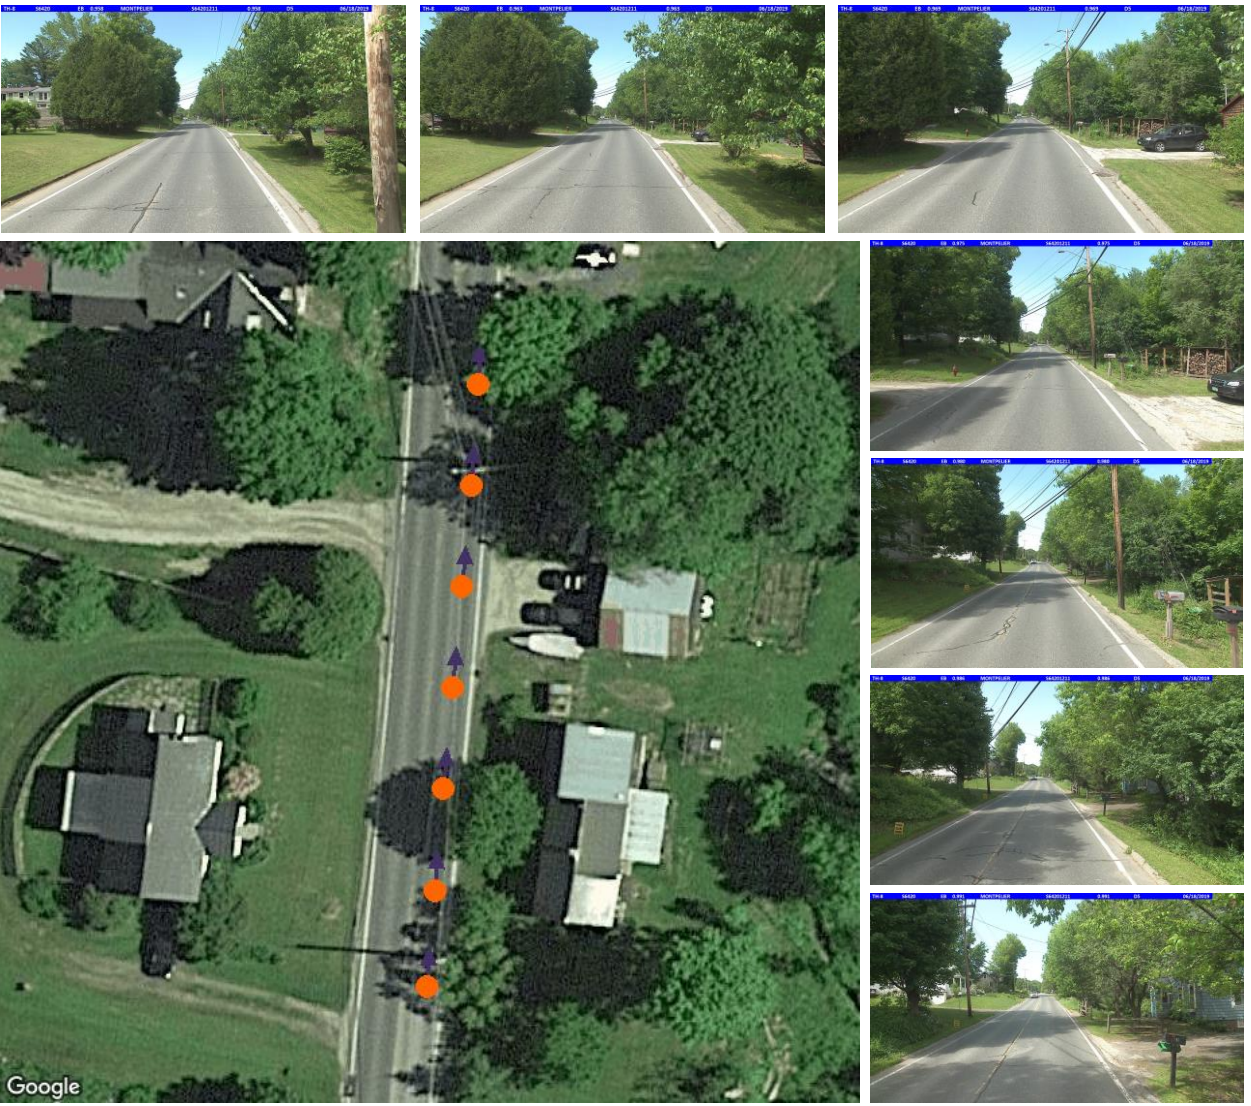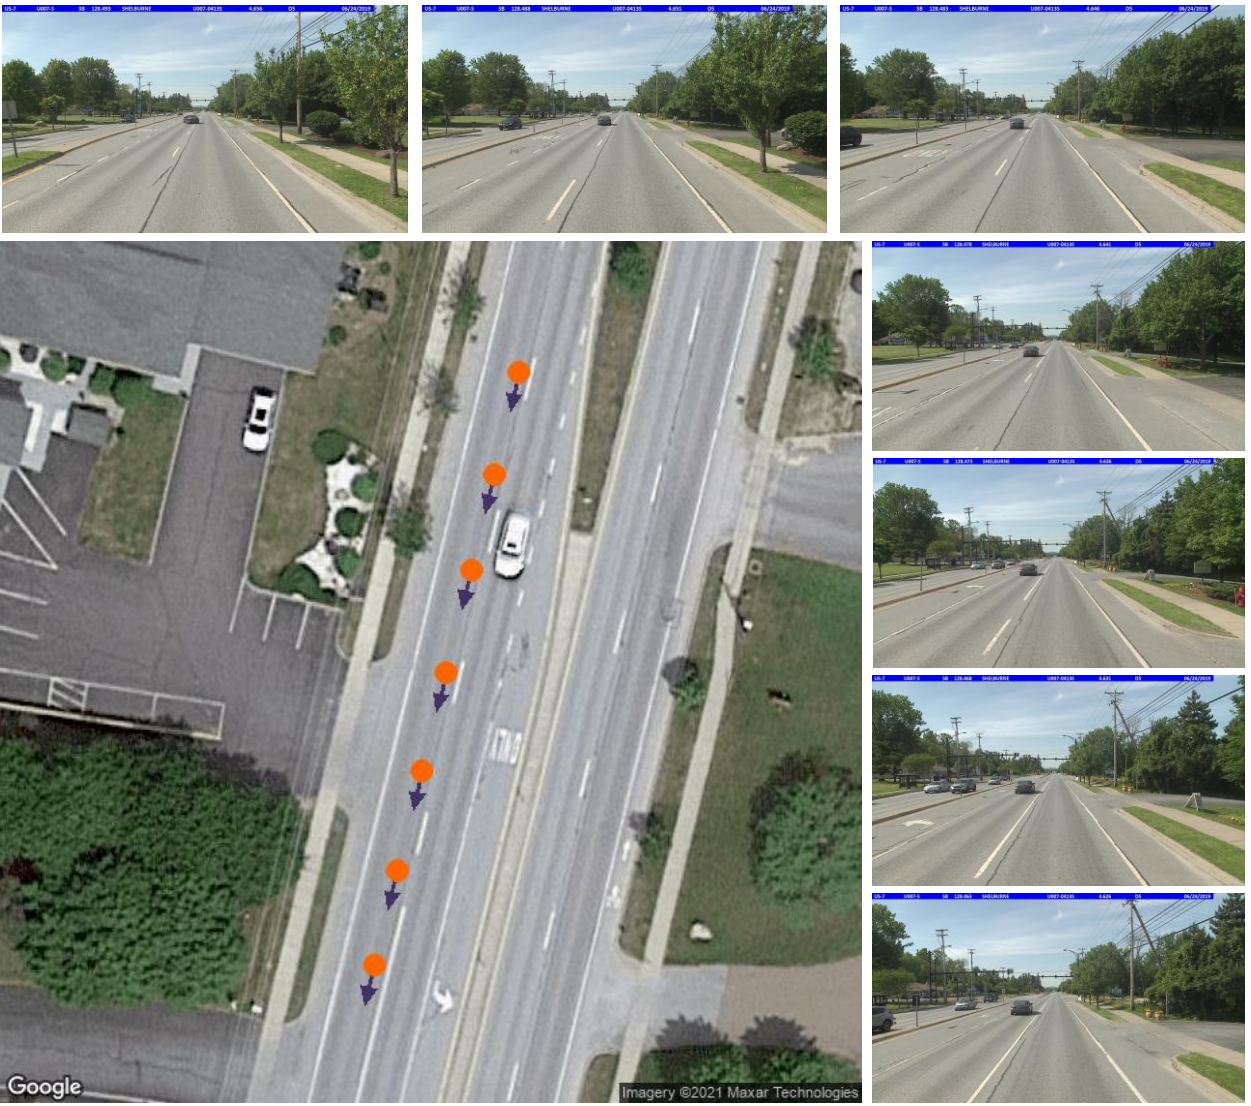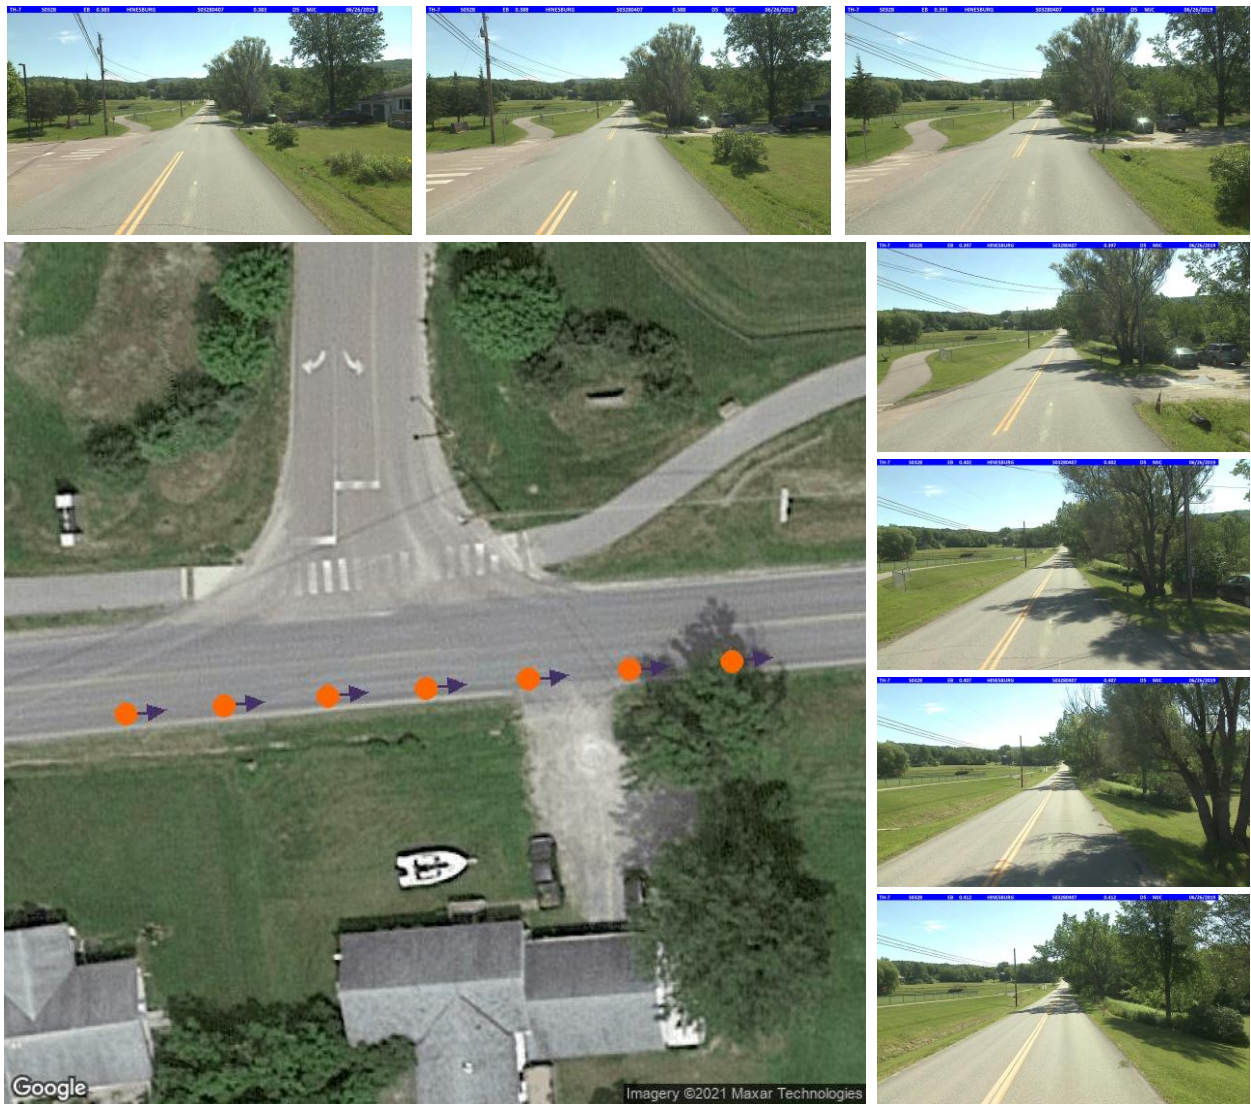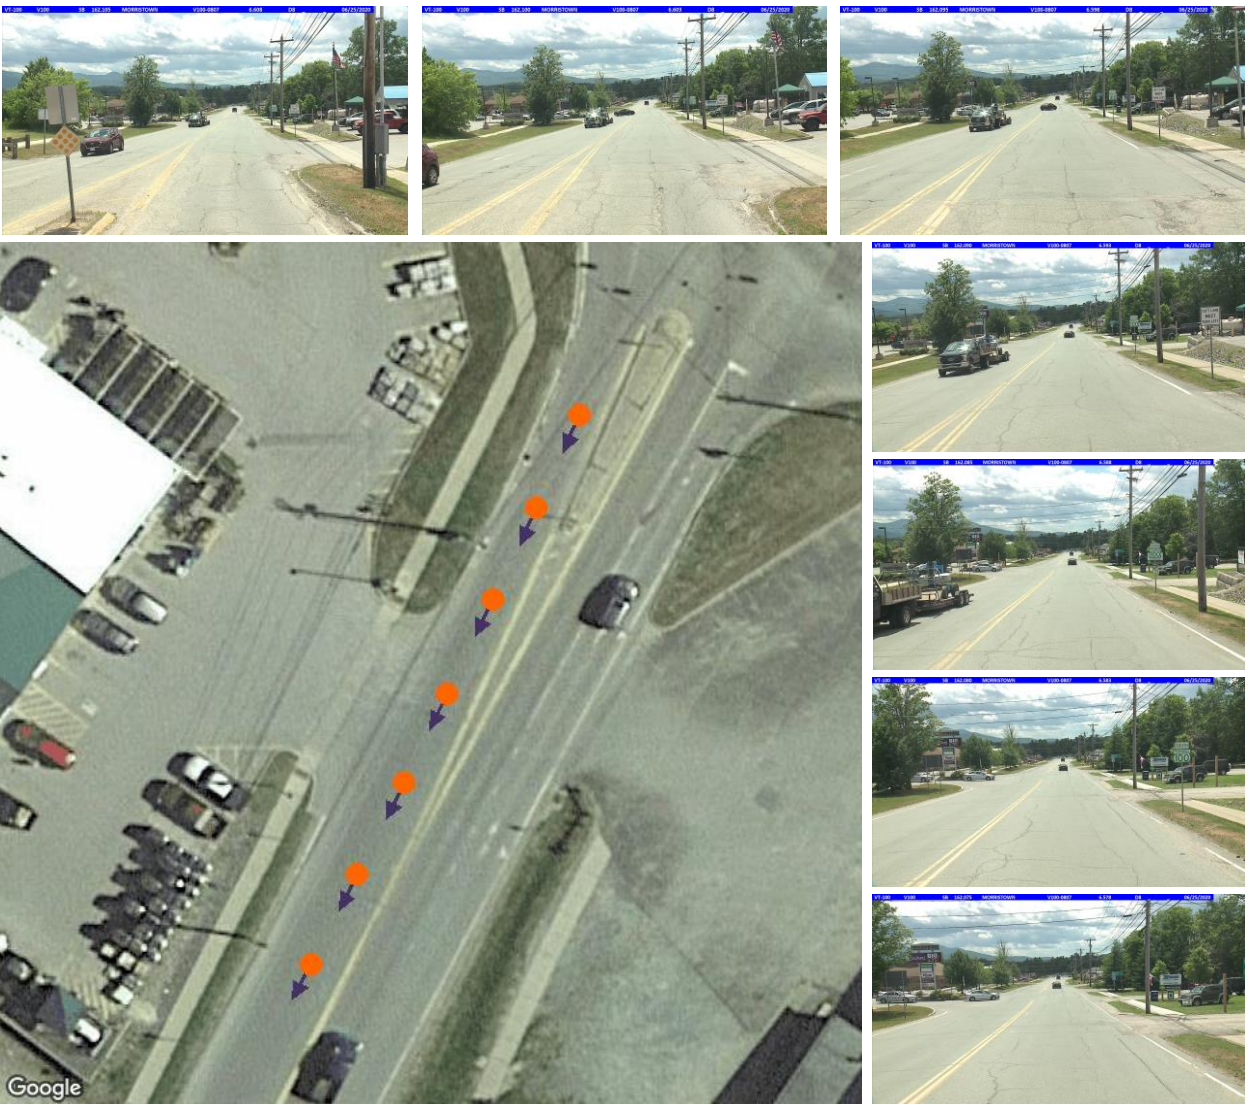

Supplement: Supplementary file 1 [file supp1.pdf]
